# Supplementary material for: Transformation optics: a time- and frequency-domain analysis of electron-energy loss spectroscopy
Source: arXiv:1605.09325 source file (2016-05-30)
Supplement: Supplementary file 1 [file Supplementary.pdf]

# Supplementary material for 'Transformation optics: A time-analysis of EELS'

May 24, 2016

## Contents

**1 EELS for non-concentric annulus** **2**
1.1 Transformation of the geomtry . . . 2
1.2 The source potential and its transformation . . . 2
1.2.1 An electron passing on the thin side of the non-concentric annulus . . . 2
1.2.2 An electron passing the crescent horizontally along its top . . . 4
1.3 Induced potentials and boundary conditions . . . 5
1.3.1 Potentials and boundary condition at the interfaces . . . 5
1.3.2 Radiative reaction boundary condition . . . 6
1.4 Power scattered . . . 8
1.5 Power absorption . . . 8
1.6 Comparison with COMSOL . . . 9
1.6.1 Vertically moving electron . . . 10
1.6.2 Horizontally moving electron . . . 11

**2 EELS for ellipse** **13**
2.1 Transformation of the geometry . . . 13
2.2 The source potential and its transformation . . . 13
2.3 Induced potentials and boundary conditions . . . 14
2.4 Power absorbed by the ellipse . . . 15
2.5 Power scattered . . . 16
2.6 Radiative reaction . . . 17
2.6.1 Fictional absorber at the origin . . . 17
2.6.2 Fictional absorber surrounding the annulus . . . 19
2.6.3 Modified expression for the $l = 1$ scattering coefficients . . . 20
2.7 Comparison with COMSOL . . . 21

**3 Permittivity of the fictional absorber** **23**

# 1 EELS for non-concentric annulus

Here we provide details on the electron energy loss calculation of a non-concentric annulus. The non-concentric annulus has permittivity $\epsilon_m$ and both its core and surrounding are assumed to have unit permittivity. We study the case of an electron passing in the vertical direction to the left of the nano-particle and in the horizontal direction along the top of the nano-particle as is shown in figure 2 in the main manuscript.

## 1.1 Transformation of the geomtry

As is shown in the main text, an annulus ($z-$frame) can be transformed to a non-concentric annulus ($z'-$frame) via a shifted inverse transformation [2]

$$\zeta' = \frac{g^2}{\zeta - x_0}, \tag{1}$$

where $z' = x' + iy'$, $z = x + iy$, $x_0 \in \mathbb{R}$ and $g \in \mathbb{R}$. The inverse transformation is given by

$$\zeta = g^2/\zeta' + x_0. \tag{2}$$

## 1.2 The source potential and its transformation

As a first step in the calculation of the energy loss and photon scattering spectrum the field associated with the exciting source has to be calculated. In the case presented here, the line electron moves on a straight trajectory and with constant velocity $c_e$. There are many ways to calculate the potential associated with this moving line charge, but the most elegant is arguably to start from the electrostatic potential of a stationary line charge and Lorentz boost it to velocity $c_e$ [3]. Here we only quote the result. In the quasi-static and non-relativistic limit, the potential for a line charge moving in the $y'-$direction at position $x' = x'_e$ is given by [7]

$$\phi' = -\frac{\lambda}{4\pi\epsilon_0\omega} e^{-i\frac{\omega}{c_e}y} e^{-|x-x'_e|\frac{\omega}{c_e}}. \tag{3}$$

### 1.2.1 An electron passing on the thin side of the non-concentric annulus

If the electron passes to the left of the crescent, i.e. $x'_e < x$ at the crescent, the potential can be written as

$$\phi^{sou} := \phi' = \frac{\lambda}{4\pi\epsilon_0\omega} \exp\left[\frac{\omega}{c_e}(iy' - x' + x'_e)\right] \tag{4}$$

$$= \frac{\lambda \exp\left[\frac{\omega}{c_e}x_e\right]}{4\pi\epsilon_0\omega} \exp\left[-\frac{\omega}{c_e}(\zeta')^*\right]. \tag{5}$$

In this form it is easily transformed from the non-concentric to the concentric frame via equation 1 as

$$\phi^{sou} = \frac{\lambda \exp\left[\frac{\omega}{c_e}x_e\right]}{4\pi\epsilon_0\omega} \exp\left[-\frac{\omega}{c_e}\left(\frac{g^2}{\zeta - x_0}\right)^*\right] \tag{6}$$

$$= \frac{\lambda \exp\left[\frac{\omega}{c_e}x_e\right]}{4\pi\epsilon_0\omega} \exp\left[-\frac{\omega}{c_e}\left(\frac{g^2}{re^{i\phi} - x_0}\right)^*\right]. \tag{7}$$

This can be expanded as

$$\phi^{sou} = \sum_{n=0}^{\infty} a_n^{s\pm} \left(\frac{r}{x_0}\right)^{\pm n} e^{\mp in\phi} \tag{8}$$

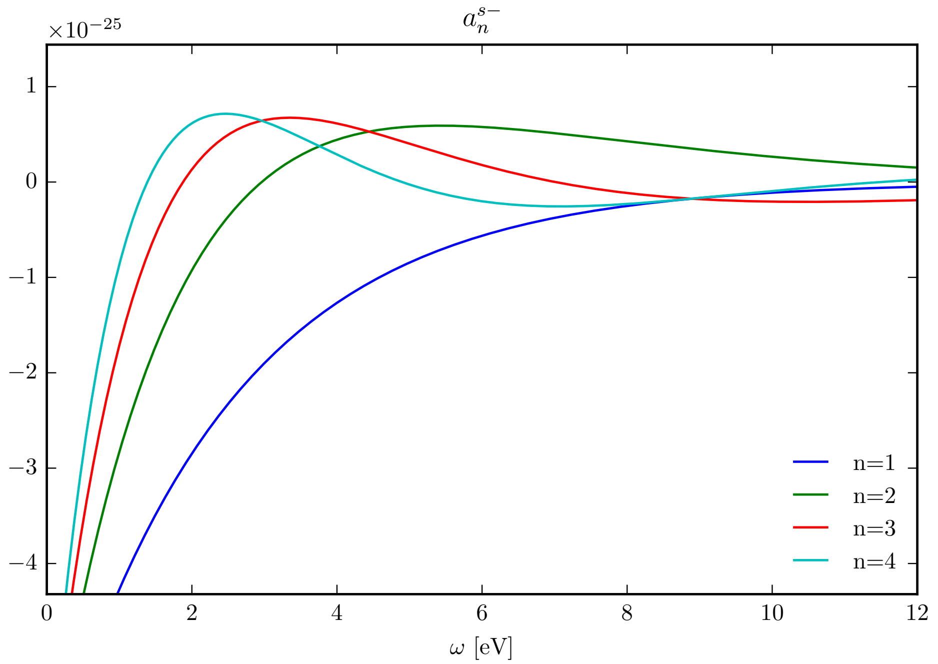


Figure 1: The source expansion coefficients $a_n^{s-}$ for the vertical case with $n = 1, 2, 3, 4$. The parameters are $\lambda = 1.602 \times 10^{-19}$, $g^2 = 2 \times 10^{-8}$, $x_0 = 1.5$, $x'_e = -0.4g^2$ and $c_e = 0.1c$. These are the same as for the green-dotted line in the electron energy loss spectrum in the main manuscript (Figure 3).

depending on whether $|x_0| > r$ or not. The expansion coefficients can be calculated as

$$a_0^{s+} = \frac{\lambda \exp\left[\frac{\omega}{c_e}x'_e + \frac{\omega g^2}{c_e x_0}\right]}{4\pi\epsilon_0\omega} \tag{9}$$

$$a_n^{s+} = \frac{\lambda \exp\left[\frac{\omega}{c_e}x'_e + \frac{\omega g^2}{c_e x_0}\right]}{4\pi\epsilon_0\omega} \sum_{k=1}^{n} \frac{(n-1)!}{k!(k-1)!(n-k)!} \left(\frac{\omega g^2}{c_e x_0}\right)^k \tag{10}$$

$$a_0^{s-} = \frac{\lambda \exp\left[\frac{\omega}{c_e}x'_e\right]}{4\pi\epsilon_0\omega} \tag{11}$$

$$a_n^{s-} = \frac{\lambda \exp\left[\frac{\omega}{c_e}x'_e\right]}{4\pi\epsilon_0\omega} \sum_{k=1}^{n} \frac{(n-1)!}{k!(k-1)!(n-k)!} \left(-\frac{\omega g^2}{c_e x_0}\right)^k, \tag{12}$$

as has been shown in [7]. Note that the scattered fields will be proportional to $a_n^{s-}$. These are damped oscillating functions of the parameter $\frac{\omega g^2}{c_e x_0}$. Their behavior is plotted against frequency in figure 1. It can be seen that the higher order modes undergo a couple of oscillations around zero before they eventually decay towards zero. This opens up the possibility for 'accidental' degeneracies, for which a zero in the source expansion coefficients coincides with the resonance frequency of that particular mode. In fact, the expansion coefficients $a_2^{s-}$ passes through zero at $\approx 3eV$. This coincides with the resonance frequency of that particular mode and explains why there is no peak in the electron energy loss spectrum at that frequency for $c_e = 0.1c$ (see figure 3 of the main manuscript).

### 1.2.2 An electron passing the crescent horizontally along its top

In the case of an electron moving horizontally but still on a straight line at $y' = y'_e$ and with constant velocity $c_e$, the source potential can simply be obtained from Eq.3 by substituting $x'_e \longrightarrow y'_e$, $x' \longrightarrow y'$ and $y' \longrightarrow x'$. Hence the source potential is given by

$$\phi' = -\frac{\lambda}{4\pi\epsilon_0\omega} e^{-i\frac{\omega}{c_e}x'} e^{-|y'-y'_e|\frac{\omega}{c_e}}. \tag{13}$$

If the electron moves along the top of the non-concentric annulus, then the fields at the annulus will be given by

$$\begin{aligned} \phi^{sou} := \phi' &= \frac{\lambda}{4\pi\epsilon_0\omega} \exp\left[\frac{\omega}{c_e}(ix' + y' - y'_e)\right] && (14) \\ &= \frac{\lambda \exp\left[-\frac{\omega}{c_e}y'_e\right]}{4\pi\epsilon_0\omega} \exp\left[i\frac{\omega}{c_e}(\zeta')^*\right] && (15) \\ &= \frac{\lambda \exp\left[-\frac{\omega}{c_e}y'_e\right]}{4\pi\epsilon_0\omega} \exp\left[i\frac{\omega}{c_e}\left(\frac{g^2}{re^{i\phi} - x_0}\right)^*\right], && (16) \end{aligned}$$

since $y'_e > y'$ at the surface of the crescent. Again, this can be expanded as [7]

$$\phi^{sou} = \sum_{n=0}^{\infty} a_n^{s\pm} \left(\frac{r}{x_0}\right)^{\pm n} e^{\mp in\phi}, \tag{17}$$

with

$$\begin{aligned} a_0^{s-} &= \frac{\lambda \exp\left[-\frac{\omega}{c_e}y'_e\right]}{4\pi\epsilon_0\omega} && (18) \\ a_n^{s-} &= \frac{\lambda \exp\left[-\frac{\omega}{c_e}y'_e\right]}{4\pi\epsilon_0\omega} \sum_{k=1}^{n} \frac{(n-1)!}{k!(k-1)!(n-k)!} \left(i\frac{\omega g^2}{c_e x_0}\right)^n && (19) \\ a_0^{s+} &= \frac{\lambda \exp\left[-\frac{\omega}{c_e}y'_e - i\frac{\omega g^2}{c_e x_0}\right]}{4\pi\epsilon_0\omega} && (20) \\ a_n^{s+} &= \frac{\lambda \exp\left[-\frac{\omega}{c_e}y'_e - i\frac{\omega g^2}{c_e x_0}\right]}{4\pi\epsilon_0\omega} \sum_{k=1}^{n} \frac{(n-1)!}{k!(k-1)!(n-k)!} \left(-\frac{i\omega g^2}{c_e x_0}\right)^k. && (21) \end{aligned}$$

Note here, that while the expansion coefficients were purely real in the case of a vertically moving electron, they now are complex. In contrast to the vertical case, this prevents the expansion coefficients to oscillate around zero. The imaginary part does show some oscillations, however real and imaginary part never vanish at the same frequency. The overall behavior of the absolute value of the expansion coefficients is thus a monotonic decrease with frequency (see figure 10). This leaves no room for 'accidental' degeneracies as could be observed for the vertical case.

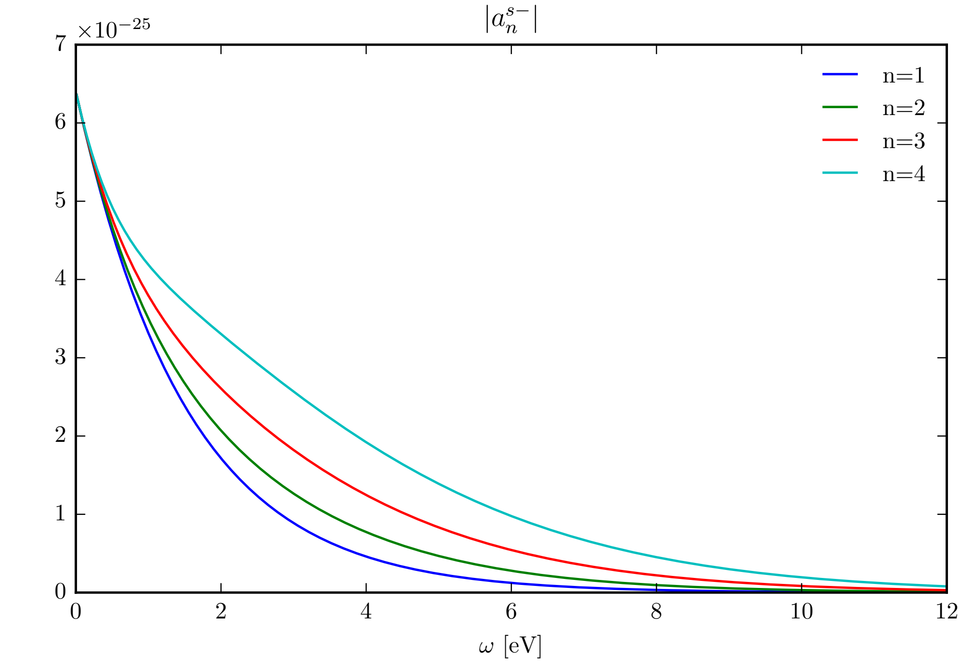


Figure 2: The absolute value of the source expansion coefficients $a_n^{s-}$ for the horizontal case with $n = 1, 2, 3, 4$. The parameters are $\lambda = 1.602 \times 10^{-19}$, $g^2 = 2 \times 10^{-8}$, $x_0 = 1.5$, $x'_e = -0.4g^2$ and $c_e = 0.1c$. These are the same as for the green-dotted line in the electron energy loss spectrum in the main manuscript (Figure 3).

## 1.3 Induced potentials and boundary conditions

### 1.3.1 Potentials and boundary condition at the interfaces

The form of the source potential in Eq.8 suggests that potentials outside and inside the annulus take the form

$$\phi_I = \sum_{n=0}^{\infty} \left[ a_n^{s+} e^{-in\phi} + (b_n + a_n^{rad+}) e^{in\phi} \right] \left( \frac{r}{x_0} \right)^n \qquad \text{for} \quad r < x_0 \tag{22}$$

$$\phi_{II} = \sum_{n=0}^{\infty} \left[ (a_n^{s-} + a_n^{rad}) \left( \frac{x_0}{r} \right)^n e^{in\phi} + b_n \left( \frac{r}{x_0} \right)^n e^{in\phi} \right] \qquad \text{for} \quad R_0 > r > x_0$$

$$\phi_{III} = \sum_{n=0}^{\infty} \left[ c_n \left( \frac{x_0}{r} \right)^n e^{in\phi} + d_n e^{in\phi} \left( \frac{r}{x_0} \right)^n \right] \qquad \text{for} \quad R_1 > r > R_0$$

$$\phi_{IV} = \sum_{n=0}^{\infty} e_n e^{in\phi} \left( \frac{x_0}{r} \right)^n \qquad \text{for} \quad R_1 > r > R_0 \tag{23}$$

where $R_0$ and $R_1$ are the inner and outer radius of the annulus, respectively. The coefficients $b_n, c_n, d_n$ and $e_n$ are the quasi-static scattering coefficients, which can be determined from the boundary conditions at the interfaces of the annulus. $a_n^{rad}$ however, encodes information about the radiative reaction of the nano-particle [5]. For now we treat $a_n^{rad}$ as known. The expansion coefficients can be determined by demanding continuity of the tangential component of the electric field and the normal component of the electric displacement field at the two interfaces (at $R_0$ and $R_1$), i.e. [3]

$$\partial_r \phi_I|_{r=R_0} = \epsilon_m \partial_r \phi_{II}|_{r=R_0} \tag{24}$$

$$\left.\frac{1}{r}\partial_\phi \phi_I\right|_{r=R_0} = \left.\frac{1}{r}\partial_\phi \phi_{II}\right|_{r=R_0} \tag{25}$$

and

$$\partial_r \phi_{III}|_{r=R_1} = \epsilon_m \partial_r \phi_{II}|_{r=R_1} \tag{26}$$

$$\left.\frac{1}{r}\partial_\phi \phi_I\right|_{r=R_1} = \left.\frac{1}{r}\partial_\phi \phi_{II}\right|_{r=R_1}. \tag{27}$$

This leads to a set of boundary equations that can be solved to give the scattering coefficients in terms of $a_n^{s-}$ and $a_n^{rad-}$,

$$\begin{pmatrix} b_n \\ c_n \\ d_n \\ e_n \end{pmatrix} = \begin{pmatrix} \frac{\left(\frac{R_0}{x_0}\right)^{-2n}(\epsilon_d-\epsilon_m)(\epsilon_d+\epsilon_m)[\left(\frac{R_0}{x_0}\right)^{2n}-\left(\frac{R_1}{x_0}\right)^{2n}]}{(\epsilon_d-\epsilon_m)^2\left(\frac{R_0}{x_0}\right)^{2n}-(\epsilon_d+\epsilon_m)^2\left(\frac{R_1}{x_0}\right)^{2n}} \\ \frac{-2\epsilon_d(\epsilon_d+\epsilon_m)\left(\frac{R_1}{x_0}\right)^{2n}}{(\epsilon_d-\epsilon_m)^2\left(\frac{R_0}{x_0}\right)^{2n}-(\epsilon_d+\epsilon_m)^2\left(\frac{R_1}{x_0}\right)^{2n}} \\ \frac{2\epsilon_d(\epsilon_d-\epsilon_m)}{(\epsilon_d-\epsilon_m)^2\left(\frac{R_0}{x_0}\right)^{2n}-(\epsilon_d+\epsilon_m)^2\left(\frac{R_1}{x_0}\right)^{2n}} \\ \frac{-4\epsilon_d\epsilon_m\left(\frac{R_1}{x_0}\right)^{2n}}{(\epsilon_d-\epsilon_m)^2\left(\frac{R_0}{x_0}\right)^{2n}-(\epsilon_d+\epsilon_m)^2\left(\frac{R_1}{x_0}\right)^{2n}} \end{pmatrix} [a_n^{s-} + a_{c,n}^{rad-}]. \tag{28}$$

#### 1.3.2 Radiative reaction boundary condition

To ensure energy conservation we need to include the effect of radiation damping into the present theory [8]. This information will be encoded into the expansion coefficients $a_n^{rad-}$. The approach presented here closely follows [1]. Imagine we enclose the crescent with a fictional absorbing material, with its boundary far away from the surface of the crescent. Then the power scattered by the crescent will be identical to the power absorbed by the fictive material due to the fields scattered of the crescent. In the annulus frame this fictive absorber transforms to an infinitesimal particle at position $x = x_0, y = 0$ (this point corresponds to infinity in the non-concentric annulus frame). It has been shown in [1] that this particle has a polarisability given by,

$$\gamma_{abs} = -\frac{i\pi^2\epsilon_0 k_0^2 g^4}{2}. \tag{29}$$

Any particle with a non-zero polarisability will acquire a dipole moment and scatter if a field is incident on it. Thus there is a multiple scattering event between the inner surface of the annulus and the fictive absorber at $x = x_0, y = 0$. It is this multiple scattering which determines the radiative reaction of the crescent. We can calculate the dipole moment of this scatterer as follows

$$\mathbf{p_{abs}} = \gamma_{abs}\mathbf{E}_{sca}(r = x_0, \phi = 0). \tag{30}$$

The scattered potential around this point is

$$\phi^{sca} = \sum_n e^{in\phi} b_n \left(\frac{r}{x_0}\right)^n \tag{31}$$

and the fields are

$$E_{sca}^r = -\sum_n \frac{n}{x_0} b_n e^{in\phi}\left(\frac{r}{x_0}\right)^{n-1} \tag{32}$$

$$E_{sca}^\phi = -\sum_n \frac{in}{x_0} b_n e^{in\phi}\left(\frac{r}{x_0}\right)^{n-1}. \tag{33}$$

Note that at $r = x_0$, $\phi = 0$ we have that $\hat{x} = \hat{r}$ and $\hat{\phi} = \hat{y}$. Thus

$$E^x_{sca} = -\sum_n \frac{n}{x_0} b_n \tag{34}$$

$$E^y_{sca} = -\sum_n \frac{n}{x_0} b_n i. \tag{35}$$

From this, the dipole moment of the fictive absorber can be induced as

$$p^x_{abs} = \frac{i\pi^2\epsilon_0 k_0^2 g^4}{2x_0} \sum_n n b_n \tag{36}$$

$$p^y_{abs} = -\frac{\pi^2\epsilon_0 k_0^2 g^4}{2x_0} \sum_n n b_n. \tag{37}$$

By demanding that the scattered field of this dipole is equal to the field generated by $a_n^{rad-}$ we can derive a relationship between $b_n$ and $a_n$. In detail,

$$\phi^{rad} = \sum_n \left(\frac{x_0}{r}\right)^n (a_n^{rad-}\cos(n\phi) + a_n^{rad-} i \sin(n\phi)) = -\frac{1}{2\pi\epsilon_0} \frac{\mathbf{p_{abs}} \cdot (\mathbf{r} - x_0\hat{x})}{r^2 + x_0^2 - 2x_0 r\cos(\phi)}. \tag{38}$$

The right hand side of this expression can be expanded as (for $r > x_0$)

$$-\frac{p^x_{abs}}{2\pi\epsilon_0 x_0} \sum_n \left(\frac{x_0}{r}\right)^n \cos(n\phi) - \frac{p^y_{abs}}{2\pi\epsilon_0 x_0} \sum_n \left(\frac{x_0}{r}\right)^n \sin(n\phi). \tag{39}$$

Hence, the radiation boundary condition reads

$$a_m^{rad} = -\frac{i\pi k_0^2 g^4}{4x_0^2} \sum_n n b_n. \tag{40}$$

Substituting for $b_n^c$ gives

$$a_m^{rad-} = -\frac{i\pi k_0^2 g^4}{4x_0^2} \sum_n \left( \frac{\left(\frac{R_0}{x_0}\right)^{-2n} (\epsilon_d - \epsilon_m)(\epsilon_d + \epsilon_m)[\left(\frac{R_0}{x_0}\right)^{2n} - \left(\frac{R_1}{x_0}\right)^{2n}]}{(\epsilon_d - \epsilon_m)^2 \left(\frac{R_0}{x_0}\right)^{2n} - (\epsilon_d + \epsilon_m)^2 \left(\frac{R_1}{x_0}\right)^{2n}} \right) n[a_n^{s-} + a_n^{rad-}] \tag{41}$$

$$= -\frac{i\pi k_0^2 g^4}{4x_0^2} \sum_n b_{2,n} n [a_n^{s-} + a_n^{rad-}], \tag{42}$$

with

$$b_{2,n} = \left( \frac{\left(\frac{R_0}{x_0}\right)^{-2n} (\epsilon_d - \epsilon_m)(\epsilon_d + \epsilon_m)[\left(\frac{R_0}{x_0}\right)^{2n} - \left(\frac{R_1}{x_0}\right)^{2n}]}{(\epsilon_d - \epsilon_m)^2 \left(\frac{R_0}{x_0}\right)^{2n} - (\epsilon_d + \epsilon_m)^2 \left(\frac{R_1}{x_0}\right)^{2n}} \right). \tag{43}$$

In matrix form this reads

$$(\mathbb{I} - \mathbf{B})\mathbf{a^{rad}} = \mathbf{B}\mathbf{a^s}, \tag{44}$$

with

$$B_{jn} = -\frac{i\pi k_0^2 g^4}{4x_0^2} b_{2,n} n \qquad \forall j. \tag{45}$$

So to determine $\mathbf{a^{rad}}$ we have to invert $(\mathbb{I} - \mathbf{B})$. Before we proceed to invert this via a numerical scheme, note that $\mathbf{B}$ can be written as

$$\mathbf{u}\mathbf{b^T}, \tag{46}$$

where $\mathbf{u}$ is the eigenvector of $\mathbf{B}$ simply consisting of a column of ones and $b_n = -\frac{i\pi k_0^2 g^4}{4x_0^2} b^c_{2,n} n$. Thus we can write

$$(\mathbb{I} - \mathbf{u}\mathbf{b}^{\mathbf{T}}). \tag{47}$$

This is called a rank-one perturbation (as $\mathbf{B}$ has rank one) to the identity and its inverse can be obtained from the Sherman-Morrison formula [9],

$$(\mathbb{I} - \mathbf{u}\mathbf{b}^{\mathbf{T}})^{-1} = \mathbb{I} + \frac{\mathbf{u}\mathbf{b}^{\mathbf{T}}}{1 - \mathbf{b}^{\mathbf{T}}\mathbf{u}}, \tag{48}$$

as can be verified by direct computation. Thus the radiative correction terms are given by

$$\mathbf{a}^{\mathbf{rad}} = \left[\left(\mathbb{I} + \frac{\mathbf{u}\mathbf{b}^{\mathbf{T}}}{1 - \mathbf{b}^{\mathbf{T}}\mathbf{u}}\right)\mathbf{u}\mathbf{b}^{\mathbf{T}}\right]\mathbf{a}^{\mathbf{s}} \tag{49}$$

$$= \left[\frac{\mathbf{u}}{1 - \mathbf{b}^{\mathbf{T}}\mathbf{u}}\right]\mathbf{b}^{\mathbf{T}}\mathbf{a}^{\mathbf{s}}. \tag{50}$$

Note that $\mathbf{u}$ is simply a column of ones, such that each element in $\mathbf{a}^{\mathbf{rad}}_{\mathbf{c}}$ is given by

$$a^{rad}_m = \frac{\mathbf{b}^{\mathbf{T}}\mathbf{a}^{\mathbf{s}}}{1 - \mathbf{b}^{\mathbf{T}}\mathbf{u}} \tag{51}$$

$$= \frac{\sum_n -\frac{i\pi k_0^2 g^4}{4x_0^2} b_{2,n} n a^{s-}_n}{1 + \sum_n \frac{i\pi k_0^2 g^4}{4x_0^2} b_{2,n} n}. \tag{52}$$

The above expression determines the radiative reaction and leads to coupling between all the modes, i.e. $b^c_1$ has now contributions from $a^s_2, a^s_3$, etc. whereas different modes were not coupled previously. With $a^{rad}_m$ known, all expansion coefficients can be determined.

## 1.4 Power scattered

As mentioned previously, the power scattered by the crescent is equal to the power absorbed by the fictional dipole absorber at $x_0$. This is given by [8]

$$P_{sca}(\omega) = \frac{\omega}{2}\mathrm{Im}(\mathbf{p} *_{\mathbf{abs}} \cdot \mathbf{E}^{\mathbf{sca}}(x_0,0)). \tag{53}$$

$$= \frac{\omega}{2}\mathrm{Im}(\gamma^*_{\mathbf{abs}} \cdot |\mathbf{E}^{sca}(x_0,0)|^2) \tag{54}$$

$$= \frac{\pi^2 \epsilon_0 k_0^2 g^4 \omega}{4}|\mathbf{E}^{sca}(x_0, 0)|^2. \tag{55}$$

$$= \frac{\pi^2 \epsilon_0 k_0^2 g^4 \omega}{2}|\sum_n \frac{n b_n}{x_0}|^2 \tag{56}$$

The formula for the power scattered by the nano-particle gives its photon scattering spectrum and can be measured in Cathodoluminescence experiments. To convert the power spectrum above to a photon number spectrum, the expression for $P_{sca}(\omega)$ has to be divided by $\hbar\omega$.

## 1.5 Power absorption

It is also possible to calculate the power absorbed by the non-concentric annulus via the resistive losses in it. Hence the power absorbed $Q(\omega)$ is given by [8],

$$Q = \frac{1}{2}\int_S dS \mathrm{Re}(\mathbf{j}^* \cdot \mathbf{E}), \tag{57}$$

where the integration region is inside the annulus. The electric field can be obtained from the potential as

$$E_r = -\partial_r \phi \tag{58}$$
$$= -\sum_{n=0}^{\infty} \left[ -nc_n \left( \frac{x_0^n}{r^{n+1}} \right) + nd_n \left( \frac{r^{n-1}}{x_0^n} \right) \right] e^{i\phi n} \tag{59}$$
$$E_\phi = -\frac{1}{r} \partial_\phi \phi \tag{60}$$
$$= -\frac{1}{r} \sum_{n=0}^{\infty} in \left[ c_n \left( \frac{x_0^n}{r^n} \right) + d_n \left( \frac{r^n}{x_0^n} \right) \right] e^{i\phi n}. \tag{61}$$

The current is related to the electric field via [3]

$$\mathbf{j} = -i\omega\epsilon_0(\epsilon_m - 1)\mathbf{E}. \tag{62}$$

Thus the radial component of the integral reads

$$j_r^* E_r = i\omega\epsilon_0(\epsilon_m^* - 1) \sum_{n=0}^{\infty} \sum_{k=0}^{\infty} \left[ -nc_n \left( \frac{x_0^n}{r^{n+1}} \right) + nd_n \left( \frac{r^{n-1}}{x_0^n} \right) \right] \left[ -k(c_k)^* \left( \frac{x_0^k}{r^{k+1}} \right) + k(d_k)^* \left( \frac{r^{k-1}}{x_0^k} \right) \right] e^{i\phi(n-k)}. \tag{63}$$

Integrating over the angular part then gives

$$\int_0^{2\pi} d\phi j_r^* E_r = 2\pi i\omega\epsilon_0(\epsilon_m^* - \epsilon_d) \sum_{n=0}^{\infty} \left[ n^2 |c_n|^2 \left( \frac{x_0^{2n}}{r^{2n+2}} \right) - 2n^2 \mathrm{Re}(d_n(c_n)^*) \frac{1}{r^2} + n^2 |d_n|^2 \left( \frac{r^{2n-2}}{x_0^{2n}} \right) \right] \tag{64}$$

Performing the radial integration from $R_0$ to $R_1$ yields

$$\int_0^{2\pi} d\phi \int r dr j_r^* E_r = 2\pi i\omega\epsilon_0(\epsilon_m^* - 1) \sum_{n=0}^{\infty} \left[ \frac{n}{2} |c_n|^2 x_0^{2n} (R_0^{-2n} - R_1^{-2n}) \right. \tag{65}$$
$$\left. - 2n^2 \mathrm{Re}(d_n(c_n)^*) \log(R_1/R_0) + \frac{n}{2} |d_n|^2 x_0^{-2n} (R_1^{2n} - R_0^{2n}) \right] \tag{66}$$

The integration for the angular fields can be carried out in a similar manner. Upon adding the two contributions the cross terms $\propto 2n^2 \mathrm{Re}(d_n(c_n)^*)$ cancel and the expression for the power absorption simplifies to

$$Q = \frac{1}{2} \int_S dS \mathrm{Re}(\mathbf{j}^* \cdot \mathbf{E}) \tag{67}$$
$$= \pi\omega\epsilon_0 \mathrm{Im}(\epsilon_m) \sum_{n=0}^{\infty} \left[ n|c_n|^2 x_0^{2n} (R_0^{-2n} - R_1^{-2n}) + n|d_n|^2 x_0^{-2n} (R_1^{2n} - R_0^{2n}) \right]. \tag{68}$$

Note that this gives only the power absorbed by the metal nano-particle, not the total energy lost by the electron. To obtain the total electron energy loss, the power scattered by the nano-particle and the power absorbed by it have to be added, i.e. the total electron energy loss spectrum as function of frequency $Q(\omega) + P_{sca}(\omega)$, has to be integrated over all frequencies.

## 1.6 Comparison with COMSOL

In this section we compare the power absorption and scattering that were obtained analytically under the electrostatic approximation with full electrodynamic simulation based on COMSOL Multiphysics. In COMSOL a moving line electron can be modeled by realising that associated with a moving line electron is a current give by [7]

$$\mathbf{j}_{e^-}(x', y', t) = \hat{y'} \lambda c_e \delta(y' - c_e t) \delta(x'). \tag{69}$$

The frequency space version of this (i.e. its Fourier transform) is given by [7]

$$\mathbf{j}_{e^-}(x', y', \omega) = \hat{y}' \frac{\lambda}{2\pi} e^{i\frac{\omega}{c_e} y'} \delta(x'). \quad (70)$$

Such a current can be modeled in COMSOL by defining a current line in 2-d, with surface current components given by Eq.70. The current line has to be placed at the position of the moving line electron. Resistive losses and scattered power are standard quantities to be obtained from COMSOL. Below is a comparison between the results from COMSOL simulations and our analytical calculations.

The results show excellent agreement between analytical calculations and numerical simulations, giving a strong indication that our theory is able to accurately predict the electron energy loss and photon scattering spectrum for a non-concentric annulus. The diameter of the annulus was approximately $\approx 20nm$.

### 1.6.1 Vertically moving electron

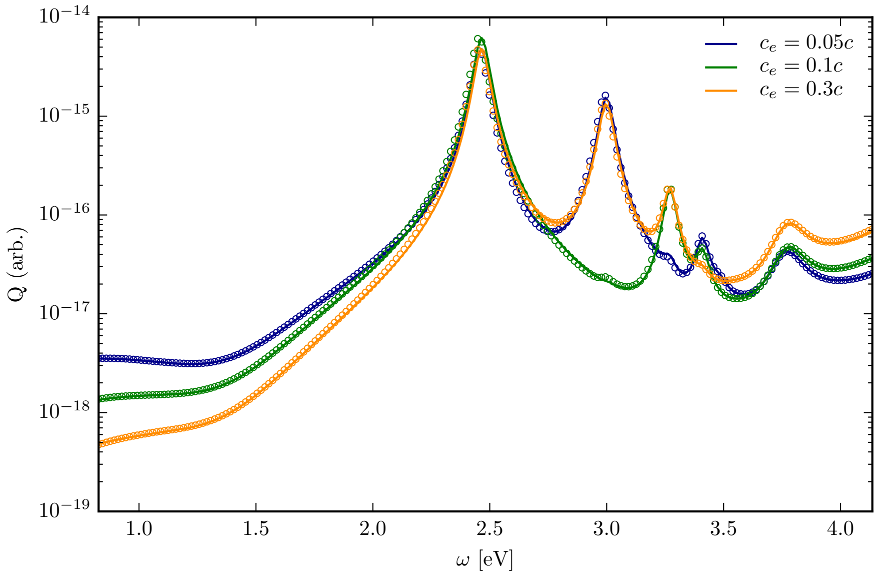


Figure 3: The resistive losses in the non-concentric annulus as calculated from Eq.68. The parameters were $\lambda = 1.602 \times 10^{-19}$, $g^2 = 2 \times 10^{-8}$, $x_0 = 1.5$ and $x'_e = -0.4g^2$. The solid lines correspond to our analytical calculations, whereas the open circles are the corresponding full electrodynamic simulations using COMSOL.

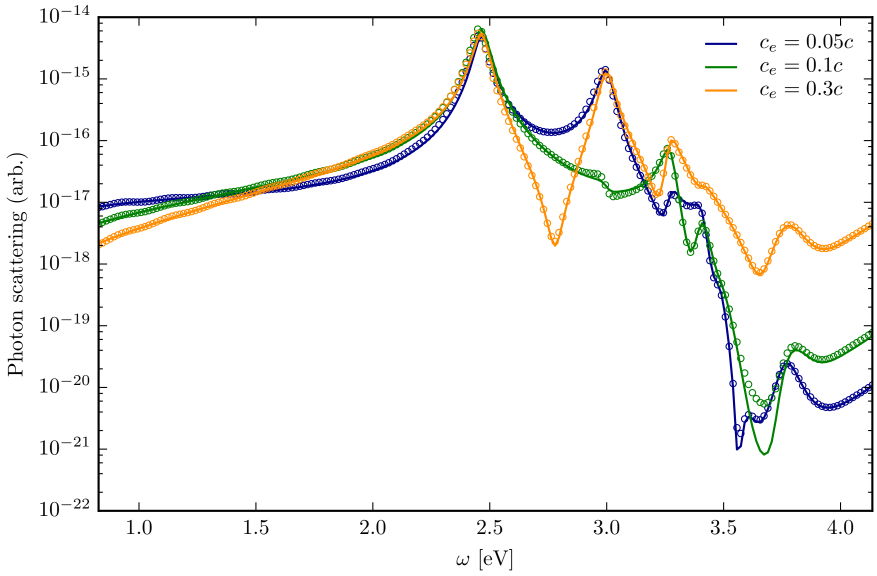


Figure 4: The photon scattering spectrum in the non-concentric annulus as calculated from Eq.56. The parameters were $\lambda = 1.602 \times 10^{-19}$, $g^2 = 2 \times 10^{-8}$, $x_0 = 1.5$ and $x'_e = -0.4g^2$. The solid lines correspond to our analytical calculations, whereas the open circles are the corresponding full electrodynamic simulations using COMSOL.

### 1.6.2 Horizontally moving electron

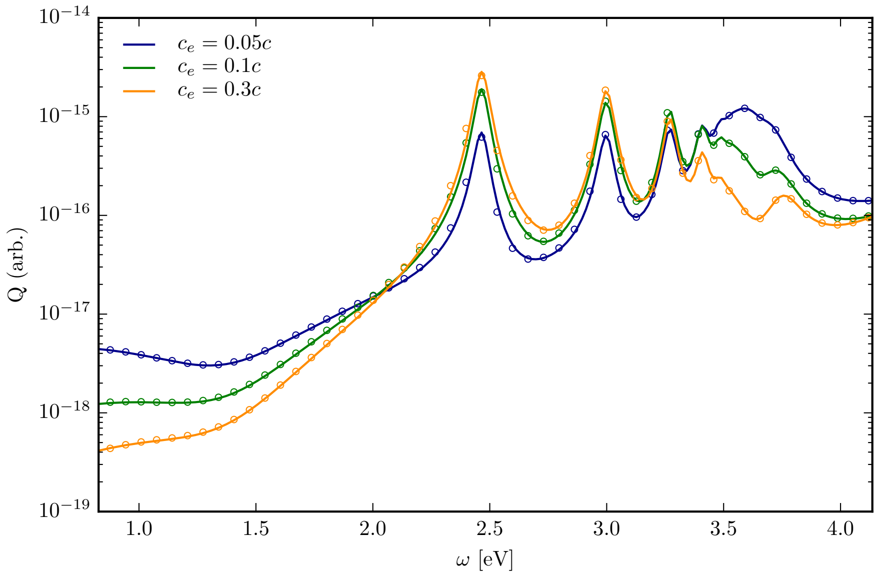


Figure 5: The resistive losses in the non-concentric annulus as calculated from Eq.68. We consider an electron moving past the top of the non-concentric annulus in the horizontal direction. The parameters were $\lambda = 1.602 \times 10^{-19}$, $g^2 = 2 \times 10^{-8}$, $x_0 = 1.5$ and $x'_e = -0.4g^2$. The solid lines correspond to our analytical calculations, whereas the open circles are the corresponding full electrodynamic simulations using COMSOL.

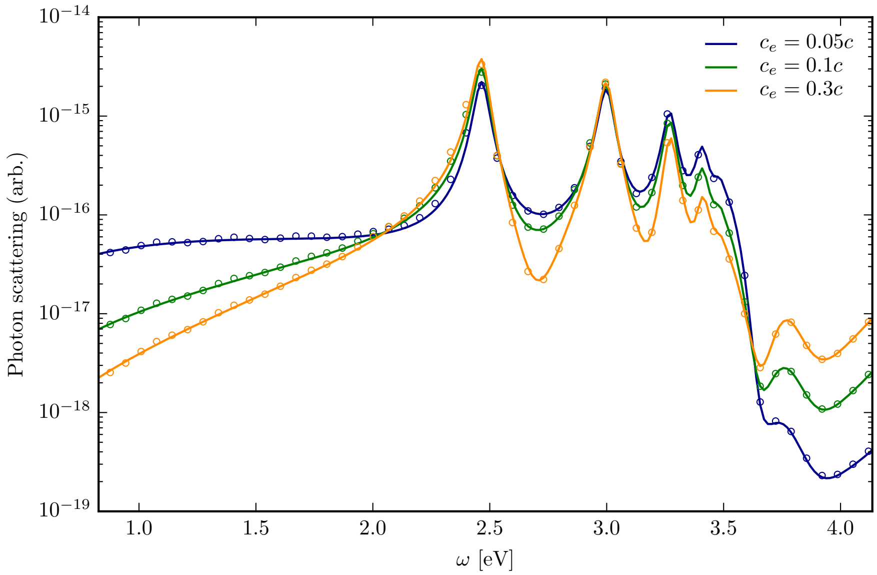


Figure 6: The photon scattering spectrum in the non-concentric annulus as calculated from Eq.56. We consider an electron moving past the top of the non-concentric annulus in the horizontal direction. The parameters were $\lambda = 1.602 \times 10^{-19}$, $g^2 = 2 \times 10^{-8}$, $x_0 = 1.5$ and $x'_e = -0.4g^2$. The solid lines correspond to our analytical calculations, whereas the open circles are the corresponding full electrodynamic simulations using COMSOL.

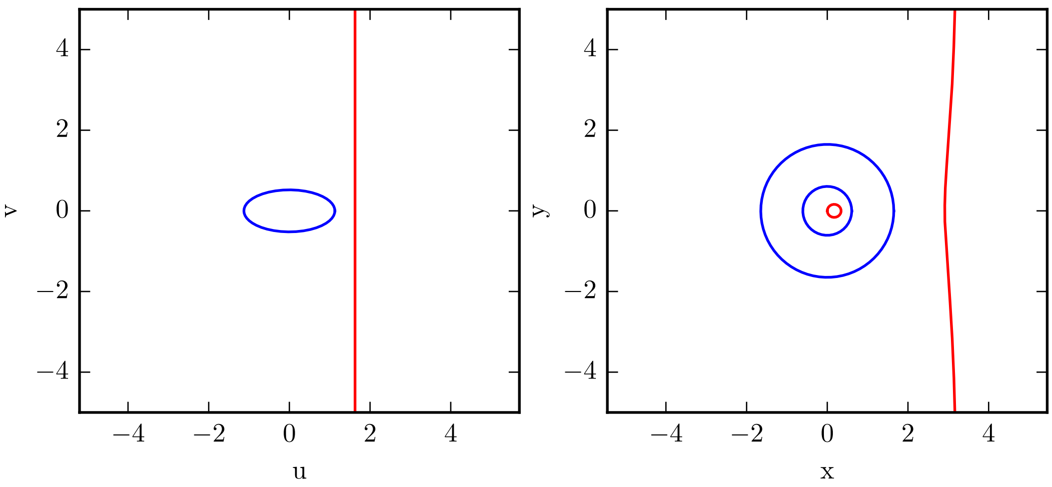


Figure 7: Schematic of the transformation of an EELS experiment for an ellipse to the equivalent annulus system.

# 2 EELS for ellipse

Here we provide details on the electron energy loss calculation for an ellipse. The ellipse has permittivity $\epsilon_m$ and is surrounded by a dielectric of unit permittivity. We study the case of an electron passing in the vertical direction to the right of the ellipse, as is shown in figure 7.

## 2.1 Transformation of the geometry

An ellipse can be transformed to an annulus using the Joukowski transformation [10, 6]

$$u + iv = \frac{c}{2}\left(x + iy + \frac{1}{x+iy}\right). \tag{71}$$

$$\zeta = \frac{c}{2}\left(z + \frac{1}{z}\right) \qquad c \in \mathbb{R}^+ \tag{72}$$

Assuming we have an ellipse with semi-major axis along the u-axis centered at the origin and a 2-D electron (i.e. line charge) moving past the ellipse at position $u = u_0$ and parallel to the v-axis. Then that situation transforms under equation 71 as is shown in figure 7. For an ellipse with semi-major axis $c\cosh(u_0)$ and semi-minor axis $c\sinh(u_0)$, the corresponding annulus will have an inner radius $R_0 = e^{-u_0}$ and an outer radius $R_1 = e^{u_0}$. For more details see [6].

## 2.2 The source potential and its transformation

As was the case for the crescent, the potential for an electron moving in the vertical $v-$direction at position $u_0$ is given by

$$\phi = \frac{\lambda}{4\pi\epsilon_0\omega}\exp\left[\frac{\omega}{c_e}(iv - |u - u_0|)\right]. \tag{73}$$

If the electron passes to the right of the ellipse, the incident potential on the ellipse is given by (since $u < u_0$)

$$\phi^{sou} = \frac{\lambda}{4\pi\epsilon_0\omega} \exp\left[\frac{\omega}{c_e}(iv + u - u_0)\right] \tag{74}$$

$$= \frac{\lambda \exp\left[-\frac{\omega}{c_e}u_0\right]}{4\pi\epsilon_0\omega} \exp\left[\frac{\omega}{c_e}\zeta\right]. \tag{75}$$

Again the transformation (Eq.71) makes it possible to write down the source potential in the annulus frame. It is given by,

$$\phi^{sou} = \frac{\lambda \exp\left[-\frac{\omega}{c_e}u_0\right]}{4\pi\epsilon_0\omega} \exp\left[\frac{\omega c}{2c_e}\left(z + \frac{1}{z}\right)\right] \tag{76}$$

$$= \frac{\lambda \exp\left[-\frac{\omega}{c_e}u_0\right]}{4\pi\epsilon_0\omega} \exp\left[\frac{\omega c}{2c_e}\left(re^{i\phi} + \frac{1}{re^{i\phi}}\right)\right] \tag{77}$$

This too, can be expanded in terms of the eigenfunctions of the annulus. Hence,

$$\phi^{sou} = \sum_{g=-\infty}^{g=\infty} a_g^s r^g e^{ig\phi}. \tag{78}$$

The expansion coefficients $a_g^s$ can be determined by expanding expanding $e^{\frac{\omega c}{2c_e} re^{i\phi}}$ and $e^{\frac{\omega c}{2c_e}\frac{1}{r}e^{-i\phi}}$. After collecting terms of equal order, the expansion coefficients can be determined as

$$a_g^s = \frac{\lambda \exp\left[-\frac{\omega}{c_e}u_0\right]}{4\pi\epsilon_0\omega} \sum_{k=0}^{\infty} \left(\frac{\omega c}{2c_e}\right)^{2k+|g|} \frac{1}{k!(k+|g|)!} \tag{79}$$

$$= \frac{\lambda \exp\left[-\frac{\omega}{c_e}u_0\right]}{4\pi\epsilon_0\omega} I_{|g|}\left(\frac{\omega c}{c_e}\right), \tag{80}$$

where $I_{|g|}(\frac{\omega c}{c_e})$ is the modified Bessel function of the first kind of order $|g|$ [**?**].

## 2.3 Induced potentials and boundary conditions

In the annulus frame we have the following source potential

$$\Phi_I^{sou} = \frac{a_0^s}{2} + \sum_{l=1}^{\infty} a_l^s r^{-l} e^{-il\phi} + \sum_{l=1}^{\infty} a_l^s r^l e^{il\phi} \tag{81}$$

This means the total potential in the three regions can be written as

$$\Phi_I = \frac{a_0^s}{2} + \sum_{l=1}^{\infty} a_l^s r^{-l}(\cos(l\phi) - i\sin(l\phi)) + \sum_{l=1}^{\infty} a_l^s r^l(\cos(l\phi) + i\sin(l\phi)) \tag{82}$$

$$+ \sum_{l=1}^{\infty} r^l(b_l^c \cos(l\phi) + b_l^s i\sin(l\phi)) \qquad \text{for } r < R_0 \tag{83}$$

$$\Phi_{II} = \frac{a_0^s}{2} + \sum_{l=1}^{\infty} r^{-l}(c_l^{c-} \cos(l\phi) + c_l^{s-} i\sin(l\phi)) + \sum_{l=1}^{\infty} r^l(c_l^{c+} \cos(l\phi) + c_l^{s+} i\sin(l\phi)) \qquad \text{for } R_0 < r < R_1 \tag{84}$$

$$\Phi_{III} = \frac{a_0^s}{2} + \sum_{l=1}^{\infty} a_l^s r^l(\cos(l\phi) + i\sin(l\phi)) + \sum_{l=1}^{\infty} a_l^s r^{-l}(\cos(l\phi) - i\sin(l\phi)) \tag{85}$$

$$+ \sum_{l=1}^{\infty} r^{-l}(d_l^c \cos(l\phi) + d_l^s i\sin(l\phi)) \qquad \text{for } R_1 < r. \tag{86}$$

The boundary conditions to determine the scattering coefficients are the same as for the crescent in Eq.24-Eq.27. The cosine-coefficients are obtained as

$$b_l^c = \left[\frac{\left((\epsilon^2-1)(R_1^{2l} - R_0^{2l}) - 4\epsilon R_1^{2l} R_0^{2l}\right)}{(\epsilon-1)^2 R_0^{2l} - (\epsilon+1)^2 R_1^{2l}} R_0^{-2l} - 1\right] a_l^s \tag{87}$$

$$c_l^{c-} = -2\frac{(\epsilon-1)R_0^{2l} R_1^{2l} + (\epsilon+1)R_1^{2l}}{(\epsilon-1)^2 R_0^{2l} - (\epsilon+1)^2 R_1^{2l}} a_l^s \tag{88}$$

$$c_l^{c+} = -2\frac{(\epsilon-1) + (\epsilon+1)R_1^{2l}}{(\epsilon-1)^2 R_0^{2l} - (\epsilon+1)^2 R_1^{2l}} a_l^s \tag{89}$$

$$d_l^c = \left[\frac{(\epsilon^2-1)(R_1^{2l} - R_0^{2l}) - 4\epsilon}{(\epsilon-1)^2 R_0^{2l} - (\epsilon+1)^2 R_1^{2l}} R_1^{2l} - 1\right] a_l^s, \tag{90}$$

while the sin-coefficients are given by

$$b_l^s = \left[\frac{\left(-(\epsilon^2-1)(R_1^{2l} - R_0^{2l}) - 4\epsilon R_1^{2l} R_0^{2l}\right)}{(\epsilon-1)^2 R_0^{2l} - (\epsilon+1)^2 R_1^{2l}} R_0^{-2l} - 1\right] a_l^s \tag{91}$$

$$c_l^{s-} = -2\frac{(\epsilon-1)R_0^{2l} R_1^{2l} - (\epsilon+1)R_1^{2l}}{(\epsilon-1)^2 R_0^{2l} - (\epsilon+1)^2 R_1^{2l}} a_l^s \tag{92}$$

$$c_l^{s+} = -2\frac{-(\epsilon-1) + (\epsilon+1)R_1^{2l}}{(\epsilon-1)^2 R_0^{2l} - (\epsilon+1)^2 R_1^{2l}} a_l^s \tag{93}$$

$$d_l^s = \left[\frac{(\epsilon^2-1)(R_1^{2l} - R_0^{2l}) + 4\epsilon}{(\epsilon-1)^2 R_0^{2l} - (\epsilon+1)^2 R_1^{2l}} R_1^{2l} + 1\right] a_l^s. \tag{94}$$

Evidently, the sin-coefficients have the same resonance condition but a slightly different sign-structure, as would be expected.

## 2.4 Power absorbed by the ellipse

As for the non-concentric annulus the power absorbed by the ellipse can be obtained from the resistive losses in it, i.e.

$$Q(\omega) = -\frac{1}{2}\text{Re}(\int_S \mathbf{j}^* \cdot \mathbf{E} dS), \tag{95}$$

where the integration is over the annulus region. The current is obtained from the electric field and the electric field from the potential. The electric field is given by

$$E_r = \sum_{l=1}^{\infty} l r^{-l-1}(c_l^{c-}\cos(l\phi) + c_l^{s-} i \sin(l\phi)) - \sum_{l=1}^{\infty} l r^{l-1}(c_l^{c+}\cos(l\phi) + c_l^{s+} i \sin(l\phi)) \tag{96}$$

$$E_\phi = \sum_{l=1}^{\infty} l r^{-l-1}(c_l^{c-}\sin(l\phi) - c_l^{s-} i \cos(l\phi)) + \sum_{l=1}^{\infty} l r^{l-1}(c_l^{c+}\sin(l\phi) - c_l^{s+} i \cos(l\phi)), \tag{97}$$

yielding currents via $\mathbf{j} = -i\omega(\epsilon - 1)\epsilon_0 \mathbf{E}$. Hence, the currents complex conjugate is given by

$$j_r^* = i\omega(\epsilon^* - 1)\epsilon_0 \left[\sum_{l=1}^{\infty} l r^{-l-1}((c_l^{c-})^*\cos(l\phi) - (c_l^{s-})^* i \sin(l\phi)) - \sum_{l=1}^{\infty} l r^{l-1}((c_l^{c+})^*\cos(l\phi) - (c_l^{s+})^* i \sin(l\phi))\right] \tag{98}$$

$$j_\phi^* = i\omega(\epsilon^* - 1)\epsilon_0 \left[\sum_{l=1}^{\infty} l r^{-l-1}((c_l^{c-})^*\sin(l\phi) + (c_l^{s-})^* i \cos(l\phi)) + \sum_{l=1}^{\infty} l r^{l-1}((c_l^{c+})^*\sin(l\phi) + (c_l^{s+})^* i \cos(l\phi))\right]. \tag{99}$$

The radial contribution to the integral comes from the term

$$j_r^* E_r = i\omega(\epsilon^* - 1)\epsilon_0 \sum_{l,g=1}^{\infty} gl \left(\left[r^{-l-1}((c_l^{c-})^*\cos(l\phi) - (c_l^{s-})^* i \sin(l\phi)) - r^{l-1}((c_l^{c+})^*\cos(l\phi) - (c_l^{s+})^* i \sin(l\phi))\right]\right. \tag{100}$$

$$\left.\times \left[r^{-g-1}(c_g^{c-}\cos(g\phi) + c_g^{s-} i \sin(g\phi)) - r^{g-1}(c_g^{c+}\cos(g\phi) + c_g^{s+} i \sin(g\phi))\right]\right). \tag{101}$$

This is quite a long expression but straightforward to integrate. Using the orthogonality of $\sin(g\phi)/\cos(g\phi)$ and the simple integral $\int_{R_0}^{R_1} dr r^{\pm 2l-1} = \frac{1}{\pm 2l - 1}\left(R_1^{\pm 2l} - R_0^{\pm 2l}\right)$, the radial contribution to the power absorption can be calculated. The angular contribution from $j_\phi^* E_\phi$ is evaluated similarly. Adding the two contributions gives the expression for the total power absorbed by the ellipse. It is given by

$$\begin{aligned} Q &= -\frac{1}{2}\text{Re}\left[i\omega(\epsilon^* - 1)\epsilon_0 \sum_{l=1}^{\infty} \frac{\pi l^2}{2l-1}(|c_l^{s+}|^2 + |c_l^{c+}|^2)\left(R_1^{2l} - R_0^{2l}\right) + \frac{\pi l^2}{-2l-1}(|c_l^{s-}|^2 + |c_l^{c-}|^2)\left(R_1^{-2l} - R_0^{-2l}\right)\right] \\ &= -\frac{\omega}{2}\pi\epsilon_0 \text{Im}(\epsilon) \sum_{l=1}^{\infty}\left[\frac{l^2}{2l-1}(|c_l^{s+}|^2 + |c_l^{c+}|^2)\left(R_1^{2l} - R_0^{2l}\right) - \frac{l^2}{2l+1}(|c_l^{s-}|^2 + |c_l^{c-}|^2)\left(R_1^{-2l} - R_0^{-2l}\right)\right]. \end{aligned} \tag{102}$$

## 2.5 Power scattered

As in the previous calculations, we can model the power scattered by the ellipse using a fictional absorber surrounding the ellipse, but far from its interface. Please note, that because the annulus to ellipse transformation is a 2-to-1 mapping, there will also be a fictional absorbing material surrounding the outer annulus and also a fictional absorber at the origin. However, the power absorbed by the fictive absorber surrounding the annulus, will be the same as the power absorbed by the absorber at the origin. Hence, dealing with the one at the origin is sufficient here, but when it comes to determining the radiative reaction the absorber surrounding the annulus will matter.

Note that in the non-concentric annulus case the fictional absorber was transformed to an absorber at position $(x, y) = (x_0, 0)$. For the ellipse, however, the fictional absorber is placed at the origin and this has important consequences on the scattering spectrum of the ellipse.

The absorber at the origin has a polarisability $\gamma_{abs}$ determined in the next section. Thus its dipole moment is given by

$$\mathbf{p_{abs}} = \gamma_{abs}\mathbf{E}_{sca}(x = 0, y = 0). \tag{103}$$

The scattered field at the origin can be found from the scattered potential as

$$\Phi_I^{sca} = \sum_{l=1}^{\infty} r^l (b_l^c \cos(l\phi) + b_l^s i \sin(l\phi)) \tag{104}$$

$$\mathbf{E}(x = 0, y = 0) = -b_1^c\hat{x} - ib_1^s\hat{y}. \tag{105}$$

Hence the dipole moment of the absorber is given by

$$\mathbf{p_{abs}} = \gamma_{abs}\left(-b_1^c\hat{x} - ib_1^s\hat{y}\right). \tag{106}$$

The power absorbed by this fictive absorber is thus

$$P_{abs} = \frac{\omega}{2}\text{Im}(\mathbf{p} *_{\mathbf{abs}} \cdot \mathbf{E^{sca}}(0, 0)) \tag{107}$$

$$= \frac{\omega}{2}\text{Im}(\gamma_{abs}^*(|b_1^c|^2 + |b_1^s|^2), \tag{108}$$

which is equal to the power scattered by the ellipse.

Note that in Eq.108 only the dipole expansion coefficients contribute to the power scattered by the ellipse. So while the near field excitation with the electron source is able to efficiently excite higher order plasmons, which manifest themselves in the absorption spectrum, the cathodoluminescence spectrum will only contain the two dipole modes. This is a consequence of the fictional absorbers position and explained via a hidden symmetry [6]. This selection rule holds strictly only in the electrostatic limit, so even for relatively small ellipses ($\approx 15nm$ semi-major axis), the quadrupole modes of the ellipse can couple to the quadrupole modes of the scattered wave and these modes become bright.

## 2.6 Radiative reaction

Figure 8 gives the transformation of the fictional absorber surrounding the ellipse. As has been mentioned previously, the power scattered to infinity by the ellipse is equal to the power absorbed by this fictional absorber. In the annulus frame, the absorber transforms to an absorber surrounding the annulus and extending to infinity, and to a small cylindrical particle at the origin. That means the power scattered by the ellipse can be calculated as the power absorbed by the fictional particle at the origin, as has been done in the previous section. For details on how to choose the permittivity of this fictional absorber see section 3.

### 2.6.1 Fictional absorber at the origin

As was the case for the non-concentric annulus, the fictional absorber at the origin will give rise to a scattered field, too. Thus, there are going to be multiple scattering events between the fictional absorber and the inner surface of the annulus. Again, this will model the radiative reaction of the ellipse. In contrast to the non-concentric annulus, this multiple scattering only effects the dipole modes, as all the other modes do not scatter under the electrostatic approximation. In the following, the change in the first order (dipole) scattering coefficients due to the multiple scattering is determined.

To model the multiple scattering correctly, the polarisability of the fictional absorber has to be determined. It can be shown that the permittivity of the fictional absorber surrounding the ellipse at position $r = a$ has to be (see Eq.181)

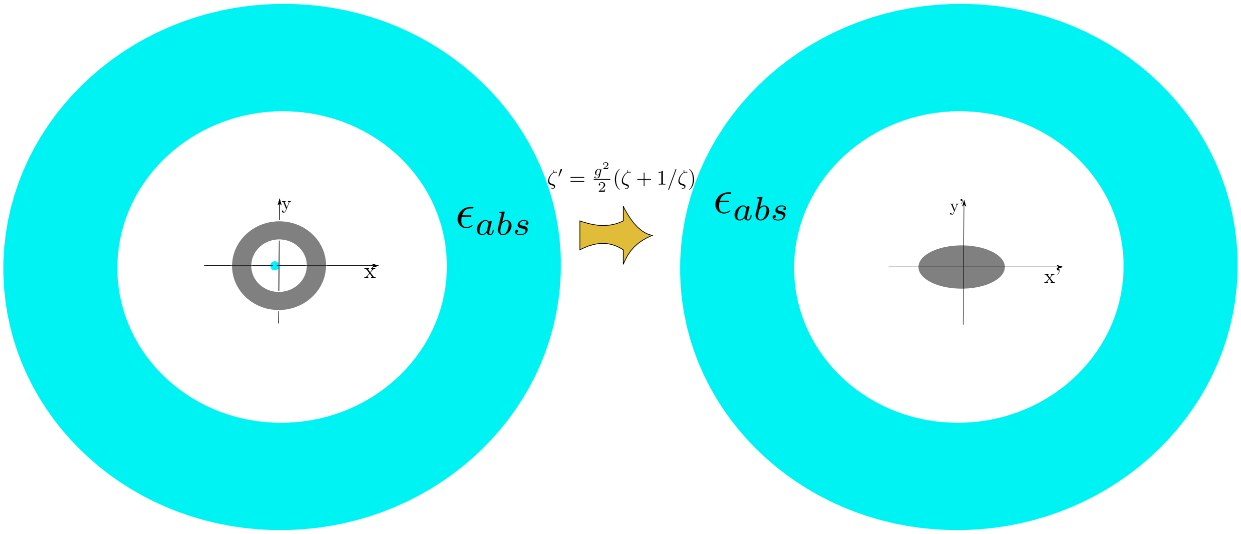


Figure 8: Schematic of the transformation of the geometry and the fictional absorber.

$$\epsilon_{abs} = 1 + 2i\pi(\frac{k_0}{2}a)^2. \tag{109}$$

This remains unchanged under a conformal transformation to the annulus frame.

In the transformed annulus frame the fictional absorber transforms to a very small cylindrical particle at the origin and a fictive absorber surrounding the whole structure. The particle at the origin must have it's radius determined by the transformation

$$z' = \frac{c}{2}(z + \frac{1}{z}). \tag{110}$$

If we are concerned with the particle near the origin the $1/z$ term is dominant and the transformation becomes

$$z' = \frac{c}{2z}. \tag{111}$$

Thus a circle of radius $r' = a$ in the ellipse's frame transforms to a circle of radius

$$r = \frac{c}{2a} \tag{112}$$

in the annulus frame.

Similarly the fictional absorber surrounding the annulus will be placed at

$$r = \frac{2a}{c}, \tag{113}$$

as in this regime $z' = \frac{c}{2}z$ holds.

The induced dipole moment of a cylindrical particle at the origin with permittivity $\epsilon_m$, radius $r = \frac{c}{2a}$ that is surrounded by vacuum is given by

$$\mathbf{p_{abs}} =2\pi\epsilon_0 \frac{c^2}{4a^2}\left(\frac{\epsilon_{abs}-1}{\epsilon_{abs}+1}\right)\mathbf{E}(\mathbf{z}=\mathbf{0}) \tag{114}$$

$$=2\pi\epsilon_0 \frac{c^2}{4a^2} i\pi(\frac{k_0}{2}a)^2\mathbf{E}(\mathbf{z}=\mathbf{0}) \tag{115}$$

$$=i\pi^2\epsilon_0\frac{c^2}{8}k_0^2\mathbf{E}(\mathbf{z}=\mathbf{0}) \tag{116}$$

$$=\gamma_{abs}\mathbf{E}(\mathbf{z}=\mathbf{0}), \tag{117}$$

where we defined the polarisability of the fictive absorber as

$$\gamma_{abs} = i\pi^2\epsilon_0\frac{c^2}{8}k_0^2. \tag{118}$$

In the above calculation we used the permittivity in Eq.109 and expanded to order $O((\frac{k_0}{2}a)^2)$. With the polarisability of the fictional absorber known, the potential scattered by it can be deduced. It is simply that of a dipole at the origin

$$\Phi_{I,rad} = \frac{1}{2\pi\epsilon_0}\frac{p_{abs,x}\cos(\phi)+p_{abs,y}\sin(\phi)}{r}, \tag{119}$$

with dipole moment

$$\mathbf{p_{abs}} = \begin{pmatrix} -\gamma_{abs}b_1^c \\ -i\gamma_{abs}b_1^s \end{pmatrix}. \tag{120}$$

This will modify the potential inside the annulus to

$$\Phi_I = \frac{a_0^s}{2} + \sum_{l=1}^{\infty} a_l^s r^{-l}(\cos(l\phi) - i\sin(l\phi)) + \sum_{l=1}^{\infty} r^l (b_l^c\cos(l\phi) + b_l^s i\sin(l\phi)) \tag{121}$$

$$+\frac{1}{2\pi\epsilon_0}\frac{p_{abs,x}\cos(\phi)+p_{abs,y}\sin(\phi)}{r} \qquad \text{for} \qquad r<R_0, \tag{122}$$

which will modify the boundary condition for the $l=1$ term, but leave all terms $l\neq 1$ unchanged.

To unambiguously determine the expansion coefficients for $l=1$ we also need to determine the effect of the fictive absorber surrounding the annulus.

### 2.6.2 Fictional absorber surrounding the annulus

The potential outside the annulus also has to be modified, since there will be a backscattering from the fictional absorber surrounding the structure. Here our main assumption is that at the interface between vacuum and the fictive absorber the only non-zero scattering coefficients are the dipole terms. I.e. the interface has to be far enough from the surface of the annulus such that all higher order modes have decayed to zero. That means we assume that the potential incident on that boundary is

$$\Phi_{II,sca}(r \longrightarrow 2a/c) = \frac{1}{r}d_1^c\cos(\phi) + \frac{1}{r}id_1^s\sin(\phi). \tag{123}$$

There will thus be a reflected potential given by

$$\Phi_{II,rad} = rR_{rad}^c\cos(\phi) + riR_{rad}^s\sin(\phi) \qquad \text{for} \quad r<\frac{2a}{c} \tag{124}$$

$$= \frac{1}{r}T_{rad}^c\cos(\phi) + \frac{1}{r}iT_{rad}^s\sin(\phi). \tag{125}$$

Matching the two expressions at the boundary gives

$$R^c_{rad} - \left(\frac{2a}{c}\right)^{-2} d^c_1 = -\epsilon_{abs} \left(\frac{2a}{c}\right)^{-2} T^c_{rad} \tag{126}$$

$$R^c_{rad} + \left(\frac{2a}{c}\right)^{-2} d^c_1 = \left(\frac{2a}{c}\right)^{-2} T^c_{rad}, \tag{127}$$

which can be solved to give

$$R^c_{rad} = \left(\frac{2a}{c}\right)^{-2} \frac{1-\epsilon_{abs}}{1+\epsilon_{abs}} d^c_1 \tag{128}$$

and identically for the sin-reflection

$$R^s_{rad} = \left(\frac{2a}{c}\right)^{-2} \frac{1-\epsilon_{abs}}{1+\epsilon_{abs}} d^s_1. \tag{129}$$

Both terms can be further reduced to

$$R^{c/s}_{rad} = -\left(\frac{2a}{c}\right)^{-2} i\pi(\frac{k_0}{2}a)^2 d^{c/s}_1 \tag{130}$$

$$= \frac{-i\pi c^2 k_0^2}{16} d^{c/s}_1. \tag{131}$$

This of course means that the boundary condition at the outer interface of the annulus has to be modified for the $l = 1$ term, as the potential there has changed to

$$\Phi_{III} = \frac{a^s_0}{2} + \sum_{l=1}^{\infty} a^s_l r^l (\cos(l\phi) + i\sin(l\phi)) + \sum_{l=1}^{\infty} r^{-l}(d^c_l \cos(l\phi) + d^s_l i \sin(l\phi)) \tag{132}$$

$$+ rR^c_{rad}\cos(\phi) + riR^s_{rad}\sin(\phi) \qquad \text{for} \qquad R_1 < r < \frac{2a}{c}. \tag{133}$$

### 2.6.3 Modified expression for the $l = 1$ scattering coefficients

As should be evident from the discussion above, the boundary conditions for the $l = 1$ term have changed. This means the expression for the $l = 1$ expansion coefficients will also be different. The new potentials for the $l = 1$term are

$$\Phi_I = a^s_1 r^{-1}(\cos(\phi) - i\sin(\phi)) + r^1(b^c_1\cos(\phi) + b^s_1 i\sin(\phi)) \tag{134}$$

$$+ \frac{1}{2\pi\epsilon_0}\frac{p_{abs,x}\cos(\phi) + p_{abs,y}\sin(\phi)}{r} \qquad \text{for } r < R_0 \tag{135}$$

$$\Phi_{II} = r^{-1}(c^{c-}_1\cos(\phi) + c^{s-}_1 i\sin(\phi)) + r^1(c^{c+}_1\cos(\phi) + c^{s+}_1 i\sin(\phi)) \qquad \text{for } R_0 < r < R_1 \tag{136}$$

$$\Phi_{III} = a^s_1 r^1(\cos(\phi) + i\sin(\phi)) + r^{-1}(d^c_1\cos(\phi) + d^s_1 i\sin(\phi)) \tag{137}$$

$$+ rR^c_{rad}\cos(\phi) + riR^s_{rad}\sin(\phi) \qquad \text{for } R_1 < r < \frac{2a}{c}. \tag{138}$$

Applying the boundary conditions in Eq.24-Eq.27 gives a set of linear equations, which can be solved using Mathematica to give

$$b_1^c = - a_1^s \left(\left[C_0(\epsilon+1)^2 R_0^2 R_1^{-2} - C_0(\epsilon-1)^2 - \left(\epsilon^2-1\right)(R_0^2 R_1^{-2}-1)R_1^{-2}\right] - 4\epsilon R_0^2 R_1^{-2}\right)/C \tag{139}$$

$$\tag{140}$$

$$c_1^{c-} = 2a_1^s R_0^2 \left(\left[C_0(1-\epsilon_0) + (1+\epsilon)R_1^{-2}\right] - \left[R_1^{-2}(C_0(1+\epsilon) + R_0^2(1-\epsilon))\right]\right)/C \tag{141}$$

$$c_1^{c+} = 2R_1^{-2} a_1^2 \left(\left[(\epsilon-1)R_0^2 R_1^{-2} - C_0(\epsilon+1)R_0^2\right] + \left[(\epsilon+1)R_0^2 - (\epsilon-1)C_0\right]\right)/C \tag{142}$$

$$\tag{143}$$

$$d_1^c = - a_1^s \left(-4\epsilon R_0^2 R_1^{-2} + a_1^s \left[C_0\left((\epsilon+1)^2 R_0^2 R_1^{-2} - (\epsilon-1)^2\right) - R_0^2\left(\left(\epsilon^2-1\right)(R_0^2 R_1^{-2}-1)\right)\right]\right)/C \tag{144}$$

$$\tag{145}$$

with the denominator given by

$$C = R_0^2 R_1^{-2}\left[(\epsilon+1)^2 - (\epsilon-1)^2 R_0^2 R_1^{-2}\right] \tag{146}$$

$$+ C_0\left[(\epsilon^2-1)(R_0^2 R_1^{-2}-1)(R_0^2 + R_1^{-2})\right] \tag{147}$$

$$+ C_0^2\left[(1+\epsilon)^2 R_0^2 R_1^{-2} - (\epsilon-1)^2\right] \tag{148}$$

and

$$C_0 = \frac{i\pi c^2 k_0^2}{16}. \tag{149}$$

Similarly, for the sin-coefficients one obtains

$$b_1^s = - a_1^s \left(-\left[C_0(\epsilon+1)^2 R_0^2 R_1^{-2} - C_0(\epsilon-1)^2 - \left(\epsilon^2-1\right)(R_0^2 R_1^{-2}-1)R_1^{-2}\right] - 4\epsilon R_0^2 R_1^{-2}\right)/C \tag{150}$$

$$\tag{151}$$

$$c_1^{s-} = 2a_1^s R_0^2 \left(-\left[C_0(1-\epsilon) + (1+\epsilon)R_1^{-2}\right] - \left[R_1^{-2}(C_0(1+\epsilon) + R_0^2(1-\epsilon))\right]\right)/C \tag{152}$$

$$c_1^{s+} = 2R_1^{-2} a_1^2 \left(-\left[(\epsilon-1)R_0^2 R_1^{-2} - C_0(\epsilon+1)R_0^2\right] + \left[(\epsilon+1)R_0^2 - (\epsilon-1)C_0\right]\right)/C \tag{153}$$

$$\tag{154}$$

$$d_1^s = - a_1^s \left(4\epsilon R_0^2 R_1^{-2} + a_1^s \left[C_0\left((\epsilon+1)^2 R_0^2 R_1^{-2} - (\epsilon-1)^2\right) - R_0^2\left(\left(\epsilon^2-1\right)(R_0^2 R_1^{-2}-1)\right)\right]\right)/C \tag{155}$$

$$\tag{156}$$

with the same denominator $C$ as for the cosine-coefficients.

The effect of this multiple scattering that led to these modified expansion coefficients is to introduce radiation damping for the dipole modes. This significantly reduces their peak heights in the scattering and absorption spectra. As mentioned previously, higher order modes are unaffected by this, as only the dipole modes of the ellipse contribute to the scattering (in the electrostatic limit).

## 2.7 Comparison with COMSOL

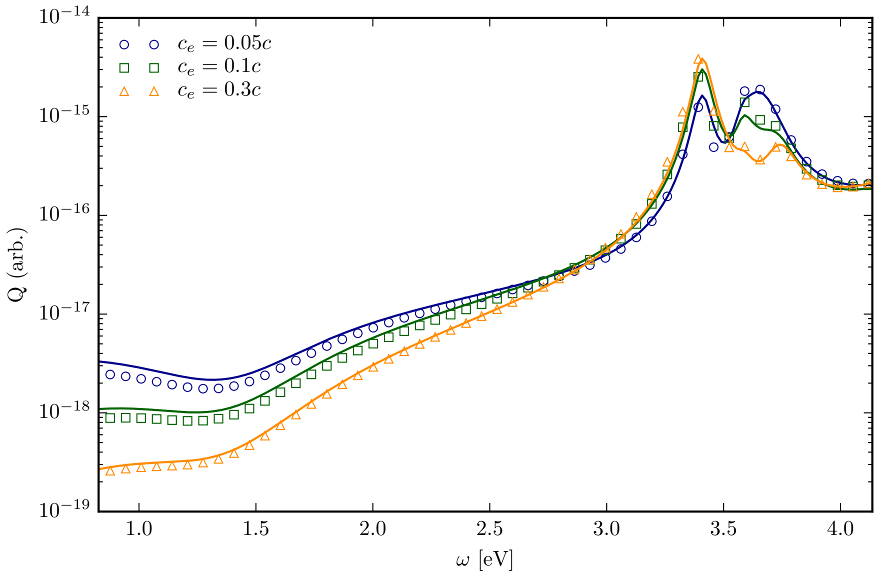


Figure 9: The resistive losses in the ellipse as calculated from Eq.102. We consider an electron moving past the right side of the ellipse in the horizontal direction. The parameters were $\lambda = 1.602 \times 10^{-19}$, $g^2 = 10^{-8}$, $u_0 = 0.4$ and the distance of the electron to the particle was $2nm$. The solid lines correspond to our analytical calculations, whereas the open circles are the corresponding full electrodynamic simulations using COMSOL.

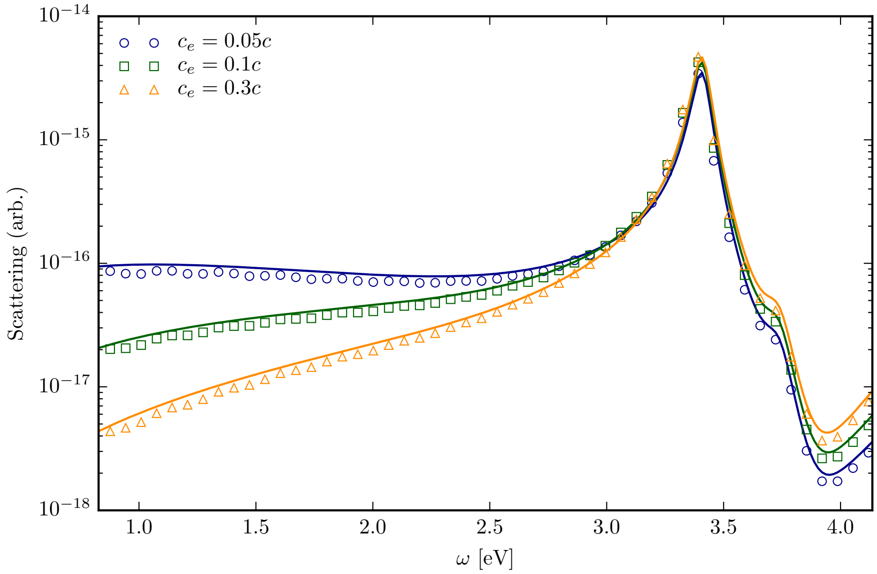


Figure 10: The photon scattering spectrum in the non-concentric annulus as calculated from Eq.102. We consider an electron moving past the right side of the ellipse in the horizontal direction. The parameters were $\lambda = 1.602 \times 10^{-19}$, $g^2 = 10^{-8}$, $u_0 = 0.4$ and the distance of the electron to the particle was $2nm$. The solid lines correspond to our analytical calculations, whereas the open circles are the corresponding full electrodynamic simulations using COMSOL.

# 3 Permittivity of the fictional absorber

Here we derive the permittivity of the fictional absorber surrounding the ellipse/non-concentric annulus. This section follows the presentation in [1] in spirit, but differs in the technical details.

The problem that has to be addressed is the following. It is known that any nano-particle that has an electric field incident on it will scatter parts of that field. The question is, how can the energy scattered to infinity by the particle be calculated within an electrostatic framework? To answer this question we first look at what happens electrodynamically.

For 2-d nano-particles smaller than the wavelength the fields scattered by them to infinity will be given by cylindrical waves to a very good approximation. A cylindrical wave with an electric field in the $x-y-$plane has a magnetic component in the z-direction. That component only needs to fulfill the scalar wave equation in cylindrical coordinates and, for outgoing waves, can be written as[4]:

$$H_z = H_0 \mathcal{H}_m(k_0 r) e^{im\phi} e^{-i\omega t}, \tag{157}$$

where $\mathcal{H}_m$ is the Hankel function of the first kind [?]. In the following we will not write the time dependence explicitly. The electric field can be obtained from [3]

$$\nabla \times \mathbf{H} = -i\omega\epsilon_0 \mathbf{E}, \tag{158}$$

$$-i\omega\epsilon_0 \mathbf{E} = \frac{1}{r}\partial_\phi H_z \hat{r} - \partial_r H_z \hat{\phi}. \tag{159}$$

Before we evaluate the derivatives we will make the near field approximation $k_0 r << 1$. In this case (for $m \geq 0$)

$$\mathcal{H}_m(k_0 r) = \begin{array}{cc} 1 + i\frac{2}{\pi}(\log(k_0 r/2) + \gamma) & for \quad m = 0 \\ \frac{1}{m!}(\frac{k_0 r}{2})^m - i\frac{(m-1)!}{\pi}(\frac{2}{k_0 r})^m & for \quad m > 0. \end{array} \tag{160}$$

The derivatives of this asymptotic form are straight forward to evaluate

$$\partial_r \mathcal{H}_m(k_0 r) = \begin{array}{cc} i\frac{2}{\pi}\frac{2}{k_0 r} & for \quad m = 0 \\ \frac{1}{(m-1)!}(\frac{k_0}{2})^m r^{m-1} + i\frac{m!}{\pi}(\frac{2}{k_0})^m r^{-m-1} & for \quad m > 0. \end{array} \tag{161}$$

So we obtain for the angular component of the electric field

$$E_\phi = \frac{H_0}{i\omega\epsilon_0} e^{im\phi} \times \left[ \begin{array}{cc} \frac{2}{\pi}\frac{2}{k_0 r} & for \quad m = 0 \\ \frac{1}{(m-1)!}(\frac{k_0}{2})^m r^{m-1} + i\frac{m!}{\pi}(\frac{2}{k_0})^m r^{-m-1} & for \quad m > 0. \end{array} \right] \tag{162}$$

and for the radial component

$$E_r = -\frac{H_0}{\omega\epsilon_0} e^{im\phi} \left[ \frac{1}{(m-1)!}(\frac{k_0}{2})^m r^{m-1} - i\frac{m!}{\pi}(\frac{2}{k_0})^m r^{-m-1} \right] \quad for \quad m > 0, \tag{163}$$

since the $\phi$-derivative of the $m = 0$ component is zero.

To model these fields in an electrostatic framework we are going to assume that the above fields are created by a radiating nano-particle, which acts as a source and the reflection of the source fields from an absorber. Our task is to find the permittivity of the absorber which gives rise to a reflection matching the above solutions. That is we assume our total field is given by

$$E^{tot} = E^{sou} + E^{sca}, \tag{164}$$

where $E^{sou}$ is the field generated by the nano-particle and $E^{sca}$ corresponds to the field reflected from by the absorber. But before we can do that we have to solve the electrostatic problem first. So we assume

that there is a source at the origin leading to fields of the form $r^{-m}$. These fields are then reflected by the absorber, which we place at $r = a$, such that $ak_0 << 1$. The reflected fields have the form $r^m$. Inside the fictive absorber we can only have fields decaying with increasing radius. Therefore we can write the electrostatic potential in the two regions

$$\Phi_I^m = (r^{-m} + Rr^m)e^{im\phi} + \Phi_0 \quad \text{for } m > 0, r < a \tag{165}$$

$$\Phi_{II}^m = Tr^{-m}e^{im\phi} \quad \text{for } m > 0, r > a \tag{166}$$

$$\Phi_I^0 = A + D\log(r) \quad \text{for } m = 0, r < a \tag{167}$$

$$\Phi_{II}^0 = T_0 \log(r) \quad \text{for } m = 0, r > a \tag{168}$$

This leads to the fields

$$E_I^\phi = -im(r^{-m-1} + Rr^{m-1})e^{im\phi} \quad \text{for } m > 0, r < a \tag{169}$$

$$E_I^r = m(r^{-m-1} - Rr^{m-1})e^{im\phi} \quad \text{for } m > 0, r < a$$

$$E_{II}^\phi = -imTr^{-m-1}e^{im\phi} \quad \text{for } m > 0, r > a$$

$$E_I^r = Tmr^{-m-1}e^{im\phi} \quad \text{for } m > 0, r > a$$

$$E_I^{0,r} = Dr^{-1} \quad \text{for } m = 0, r < a$$

$$E_I^{0,r} = T_0 r^{-1} \quad \text{for } m = 0, r > a.$$

At the boundary between the two media ($r = a$) the tangential component of the electric and the normal component of the displacement field have to be continuous [3]. This gives

$$(a^{-m-1} + Ra^{m-1}) = Ta^{-m-1} \tag{170}$$

$$(a^{-m-1} - Ra^{m-1}) = \epsilon_{abs} Ta^{-m-1} \tag{171}$$

or

$$1 + Ra^{2m} = \frac{1}{\epsilon_{abs}}(1 - Ra^{2m}) \tag{172}$$

$$\epsilon_{abs} = \frac{(1 - Ra^{2m})}{(Ra^{2m} + 1)} \tag{173}$$

$$R = a^{-2m}\frac{1 - \epsilon_{abs}}{1 + \epsilon_{abs}}. \tag{174}$$

For the zero order mode we only have one equation and thus cannot determine D unambiguously, here we have

$$D = T_0 \epsilon_{abs}. \tag{175}$$

The task is now to match the electrostatic solution to the electrodynamic one. This will yield a condition on the permittivity of the absorber $\epsilon_{abs}$. We can see that we cannot match the $m = 0$ mode to the electrodynamic solution because there $E_\phi^{dynamic} \neq 0$, whereas $E_\phi^{static} = 0$. The other modes can be matched, however. The resulting reflection coefficient will depend on $m$. So the permittivity of the absorber would also have to depend on $m$. To match the coefficients in front of $r^{-m-1}$ between the electrostatic and electrodynamic case we set $H_0$ to be

$$H_0^m = -i\omega\epsilon_0 m \frac{\pi}{m!}(\frac{2}{k_0})^{-m}. \tag{176}$$

Then equating the electrodynamic (Eq.162) and electrostatic $E_\phi$ (Eq.169) gives the value for $R$ (we could equally well match $E_r$)

$$-ime^{im\phi}\left[\frac{-i\pi}{m!(m-1)!}(\frac{k_0}{2})^{2m}r^{m-1}+r^{-m-1}\right]=-im(r^{-m-1}+Rr^{m-1})e^{im\phi} \tag{177}$$

$$R=\frac{-i\pi}{m!(m-1)!}(\frac{k_0}{2})^{2m}. \tag{178}$$

This can now be used to determine the permittivity of the fictive absorber from Eq.174

$$\epsilon_{abs}^{m}=\frac{1-\frac{-i\pi}{m!(m-1)!}(\frac{k_0}{2}a)^{2m}}{1+\frac{-i\pi}{m!(m-1)!}(\frac{k_0}{2}a)^{2m}}. \tag{179}$$

For the first order mode $m=1$, this becomes

$$\epsilon_{abs}^{1}=\frac{1+i\pi(\frac{k_0}{2}a)^2}{1-i\pi(\frac{k_0}{2}a)^2} \tag{180}$$

$$\approx 1+2i\pi(\frac{k_0}{2}a)^2-2\pi^2(\frac{k_0}{2}a)^4+O((\frac{k_0}{2}a)^6). \tag{181}$$

This means we can model scattered light propagating to infinity by placing a fictional absorber around the scatterer that has a permittivity given by Eq.181. There are however constraints on where to place that fictional absorber. On the one hand it has to be in the near field such that $k_0a << 1$ holds. On the other hand it has to be far enough from the surface of the particle such that only the first order mode is present in the fields that reach the absorber. The energy absorbed by the fictional absorber is then identical to the energy scattered to infinity by the nano-particle. This approach also allows to take radiation damping into account. This can be done by solving the multiple scattering problem between the nano-particle and the fictive absorber, as has been shown above.

# References


[1] A. Aubry, D. Lei, S. A. Maier, and J. B. Pendry. Conformal transformation applied to plasmonics beyond the quasistatic limit. *Phys. Rev. B*, 82:205109, Nov 2010.

[2] A. Aubry and J. B. Pendry. *Active Plasmonics and Tuneable Plasmonic Metamaterials*, chapter 4, pages 105–152. John Wiley & Sons, Inc., 2013.

[3] John D. Jackson. *Classical Electrodynamics.* Wiley, third edition, August 1998.

[4] J.A. Kong. *Electromagnetic Wave Theory.* EMW Publishing, 6th edition edition, 2005.

[5] Matthias Kraft, Yu Luo, S. A. Maier, and J. B. Pendry. Designing plasmonic gratings with transformation optics. *Physical Review X*, 5(3):1–9, 2015.

[6] Matthias Kraft, J. B. Pendry, S. A. Maier, and Yu Luo. Transformation optics and hidden symmetries. *Phys. Rev. B*, 89:245125, Jun 2014.

[7] Yu Luo, Matthias Kraft, and J.B. Pendry. Harnessing transformation optics for understanding electron energy loss and cathodoluminescence. *submitted to PNAS*, May 2016.

[8] L. Novotny and B. Hecht. *Principles of Nano-Optics.* Cambridge University Press, 2006.

[9] William H. Press, Saul A. Teukolsky, William T. Vetterling, and Brian P. Flannery. *Numerical Recipes 3rd Edition: The Art of Scientific Computing.* Cambridge University Press, 3 edition, 2007.

[10] Roland Schinzinger and Patricio A. A. Laura. *Conformal Mapping - Methods and Applications*. Dover Publications, Inc, Minealo, New York, 2003.
